# Supplementary material for: Generalized Many-Body Expanded Full Configuration Interaction Theory
Source: arXiv:1910.03527 ancillary file (2019-12-11)
Supplement: Supplementary file 1 [file si.pdf]

# Supporting Information: Generalized Many-Body Expanded Full Configuration Interaction Theory

Janus J. Eriksen*,† and Jürgen Gauss*,‡

†*School of Chemistry, University of Bristol, Cantock's Close, Bristol BS8 1TS, United Kingdom*

‡*Institut für Physikalische Chemie, Johannes Gutenberg-Universität Mainz, Duesbergweg 10-14, 55128 Mainz, Germany*

E-mail: janus.eriksen@bristol.ac.uk; gauss@uni-mainz.de

# 1 Total Energies (Results in $E_{\mathrm{H}}$)

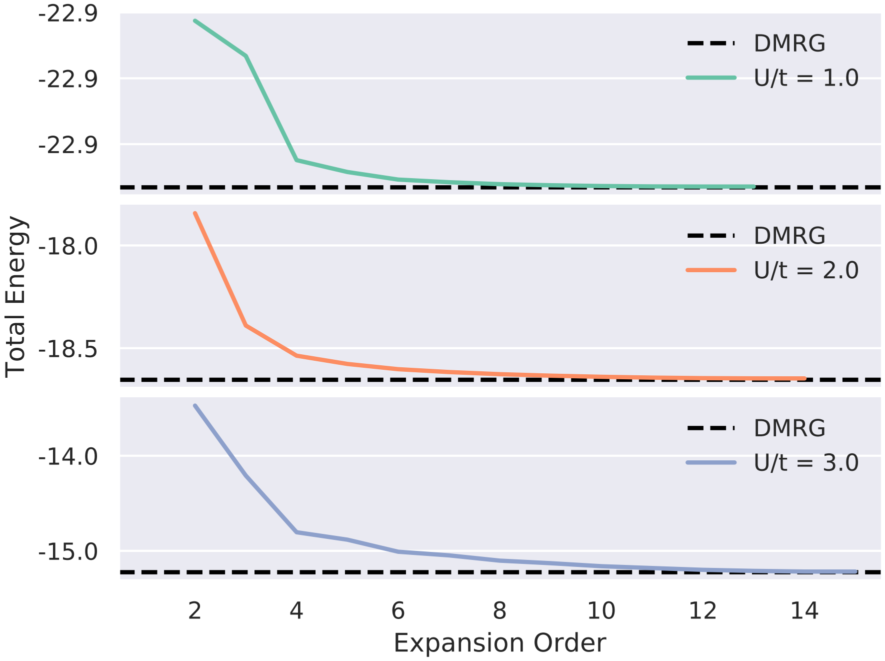


Figure S1: Convergence of MBE-FCI for the 22-site 1-dimensional Hubbard model.

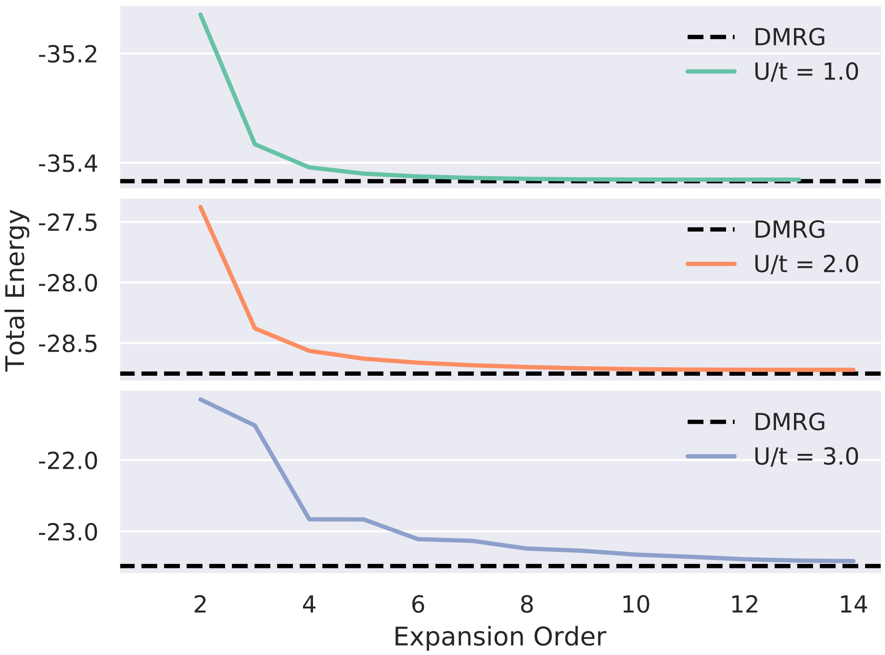


Figure S2: Convergence of MBE-FCI for the 34-site 1-dimensional Hubbard model.

Table S1: Results/site for the 1-dimensional Hubbard model at half-filling ($a = 5.0$).

| $U/t$ | $N_{\mathrm{sites}}$ | DMRG[S1] | MBE-FCI |
|---|---|---|---|
| 1.0 | 6 | −1.1002 | −1.100193 |
| 1.0 | 10 | −1.0614 | −1.061441 |
| 1.0 | 22 | −1.0447 | −1.044645 |
| 1.0 | 34 | −1.0422 | −1.042082 |
| 1.0 | 46 | −1.0414 | −1.041247 |
| 2.0 | 6 | −0.90158 | −0.901576 |
| 2.0 | 10 | −0.86384 | −0.863842 |
| 2.0 | 22 | −0.84791 | −0.847609 |
| 2.0 | 34 | −0.84567 | −0.844756 |
| 2.0 | 46 | −0.84500 | −0.843950 |
| 3.0 | 6 | −0.73890 | −0.738892 |
| 3.0 | 10 | −0.70461 | −0.704606 |
| 3.0 | 22 | −0.69203 | −0.691726 |
| 3.0 | 34 | −0.69073 | −0.688701 |
| 3.0 | 46 | −0.69040 | −0.686688 |

Table S2: Absolute deviation (in m$E_{\mathrm{H}}$/site) and relative recovery (in %) of DMRG reference results for the 1-dimensional Hubbard model with $n$ sites.

| $U/t$ | $n = 6$ | $n = 10$ | $n = 22$ | $n = 34$ | $n = 46$ |
|---|---|---|---|---|---|
| 1.0 | 0.00 | 0.00 | 0.03 | 0.09 | 0.10 |
| | (100.00) | (100.00) | (100.00) | (99.99) | (99.99) |
| 2.0 | 0.00 | 0.00 | 0.30 | 0.92 | 1.05 |
| | (100.00) | (100.00) | (99.96) | (99.89) | (99.88) |
| 3.0 | 0.00 | 0.00 | 0.30 | 2.03 | 3.71 |
| | (100.00) | (100.00) | (99.96) | (99.71) | (99.46) |

Table S3: Results for the chromium dimer.

| Method | Energy |
|---|---|
| RHF | −2085.572971 |
| CCSD(T) | −2086.422229 |
| CCSDTQ | −2086.430244 |
| DMRG | −2086.444784 |
| MBE-FCI (RHF MOs) – $a = 5.0$ | −2086.446330 |
| MBE-FCI (CCSD NOs) – $a = 5.0$ | −2086.442548 |
| MBE-FCI (CCSD NOs) – $a = 2.5$ | −2086.444961 |

Table S4: Results for the benzene molecule ($a = 5.0$).

| Method | Energy |
|---|---|
| RHF | −230.721905 |
| CCSD(T) | −231.581328 |
| CCSDTQ | −231.584190 |
| MBE-FCI (CCSD NOs) | −231.584300 |
| MBE-FCI (PM MOs) | −231.588965 |

# References

(S1) Private correspondence with Prof. Sandeep Sharma of the University of Colorado Boulder.
